# Supplementary material for: NOD-TAMP: Generalizable Long-Horizon Planning with Neural Object Descriptors
Source: arXiv:2311.01530 source file (2024-10-05)
Supplement: Supplementary file 1 [file Appendix.tex]

\newpage\hbox{}\thispagestyle{empty}\newpage
\appendix

\subsection{Real-world Experiments}

\begin{figure*}[t]
\begin{center}
    \includegraphics[width=1\linewidth]{images/real_res.pdf}
    % \vspace{-5pt}
  \end{center}
  \caption{\textbf{Real-world Results.} Key frames of three task execution processes.}
  \label{fig:real_res}
  % \vspace{-10pt}
\end{figure*}

We demonstrate deploying our method on a real Franka Emika Panda robot in Fig.~\ref{fig:real_res}. The system perceives the scene with an Intel RealSense D435 camera and uses color segmentation to extract the target objects. The system then transfers the perceived scene into a simulated environment to perform planning. We execute trajectories using open-loop control and track the generated trajectory with a joint impedance controller~\cite{hogan1985impedance} operating at a frequency of 20 Hz.

For the ClearTable task, the major failures are that the mug is not stably grasped by gripper, and the mug is slipped out during the movement. For the Serve Food task, we noticed the error caused by the perception pipeline, since the food box is almost at the size of maximal gripper distance, the robot needs to precisely align its hand pose in order to grasp the object. Additionally, task failures resulting from dynamic factors and unforeseen events were noted, such as the possibility of a bowl being flipped due to a dropping box. Incorporating task execution monitoring and re-planning capabilities has the potential to address these challenges effectively.

\subsection{Computation Efficiency Analysis}

% \begin{figure}[ht!]
%   \begin{center}
%     \includegraphics[width=1.\linewidth]{rss24/images/time_dist.pdf}
%   \end{center}
%   \caption{\textbf{Time Complexity Analysis}. \shuo{add details}}
%   \label{fig:time_dist}
%   \vspace{-10pt}
% \end{figure}

\begin{figure}[ht!]
  \begin{center}
    \includegraphics[width=1.\linewidth]{rss24/images/speed.pdf}
  \end{center}
  \caption{\textbf{Time v.s. Trajectory Lengths}. We show the running speed of our full system for a two stage task. \textbf{TA} is short for trajectory adaptation, \textbf{CT \& SR} is short for constraint transfer and skill reasoning. \textbf{Tr} is short for trajectory tracking.}
  \label{fig:time_dist}
  \vspace{-10pt}
\end{figure}

We show the speed analysis of our system in Fig.~\ref{fig:time_dist}. We evaluate our system using a two-stage task that involves skill chaining and reasoning, and we quantify the time required for each component in our pipeline. We observed that the primary time-consuming aspect is trajectory adaptation, which involves optimizing individual poses to align with the reference trajectory feature. While many routine tasks can be accomplished with coarse trajectories (e.g., less than 10 poses in our experiments), the time overhead could become a bottleneck for tasks that necessitate dense skill trajectory. This issue could potentially be mitigated by utilizing lightweight neural networks for feature encoding and leveraging more efficient optimization techniques.

% \subsection{Task and Demonstration Details}
% Explain each task in LIBERO benchmark. show task init and goals.

\subsection{Skill Demonstration Extraction and Skill Representation}
% how to segment skills, how to represent constraints
Here we provide additional detail on segmenting skill demonstrations and representing skills in \Ours to supplement Sec. III.B and IV.B-C in the main text. To segment skill-level demonstrations from a longer task demonstration, we identify kinematic alterations (e.g., gripper open / close and contact event) through detecting object contacts and pinpoint the time step at which these changes occur to establish the boundaries of each skill. Data sources such as LIBERO often contain noisy actions such as repeated grasps and accidental contacts. This requires us to manually inspect and filter out the low quality skill demonstrations. To facilitate transit and transfer motion, we further trim the skill demonstrations to segments that involve contact. In our implementation, we simply select the 50 steps before contact. Further discussion is included in Sec. IV.C of the main text. We expect future works to further automate this process through learning-based trajectory segmentation. 

\begin{figure}[h]
  \begin{center}
    \includegraphics[width=0.9\linewidth]{rss24/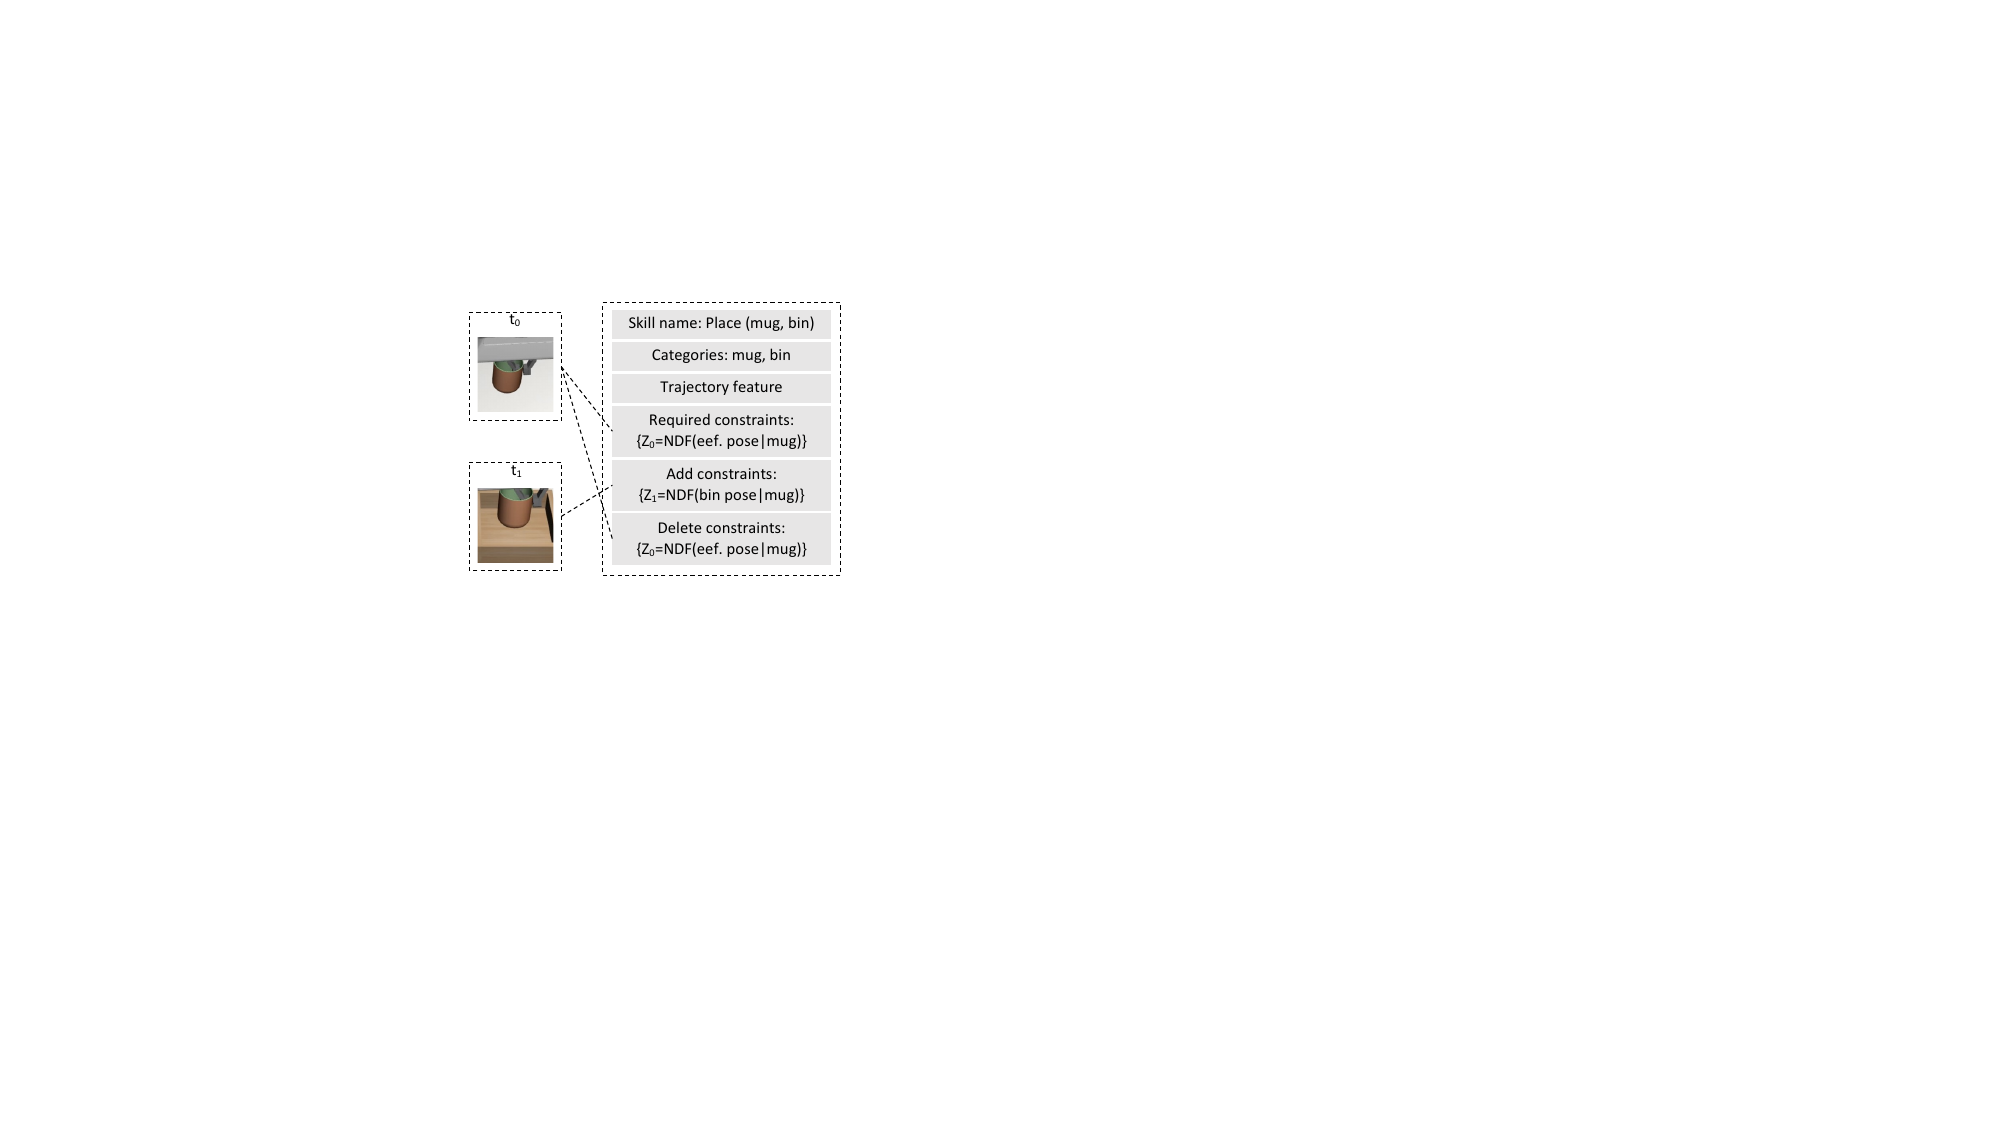}
  \end{center}
  \caption{\textbf{Skill Representation}. We show an example of how we represent the skills in \Ours.}
  \label{fig:skill_repr}
  \vspace{-10pt}
\end{figure}

Fig.~\ref{fig:skill_repr} further illustrates how a skill is represented in the skill planning step (Sec. III.B). During skill planning, a candidate skill is considered as executable only if the current acquired constraints (which are the accumulation of add constraints of all selected skills in current partial plan during the search process) include the required constraints of the candidate skill, and the compatibility score is evaluated as the feature distance between the two matched constraints.

\subsection{NDF Training}
% talk about NDF training, for libero objects, data augmentation
To enhance the generalizability of our system across various objects in the LIBERO benchmark, we extract 3D models from the LIBERO assets and utilize them to create the training dataset for the NDF model in \Ours. In line with the approach outlined by Simeonov et al.~\cite{simeonovdu2021ndf}, we adopt the same model architecture and learning hyperparameters, with learning rate of 0.0001 and batch size 16. The model is optimized using Adam optimizer~\cite{kingma2014adam} and trained for 80k epochs. We employ 3D occupancy prediction as a pre-training task to acquire object descriptor features, and we randomly rotate and scale the object model and the corresponding ground-truth to make the learned model more robust to various shapes.

\subsection{More Qualitative Evaluations}
We visualize some execution processes of LIBERO tasks in Fig.~\ref{fig:libero_qual}. The typical failure modes of our approach include gripper collision with a tight cabinet drawer, or object slippery due to sub-optimal grasp poses. We noticed that our system highly depends on the quality of the reference demos, so some of the failures can be improved through providing high-quality demos, incorporating replanning capability would also make the system more robust.

\begin{figure*}[h]
\begin{center}
    \includegraphics[width=1\linewidth]{rss24/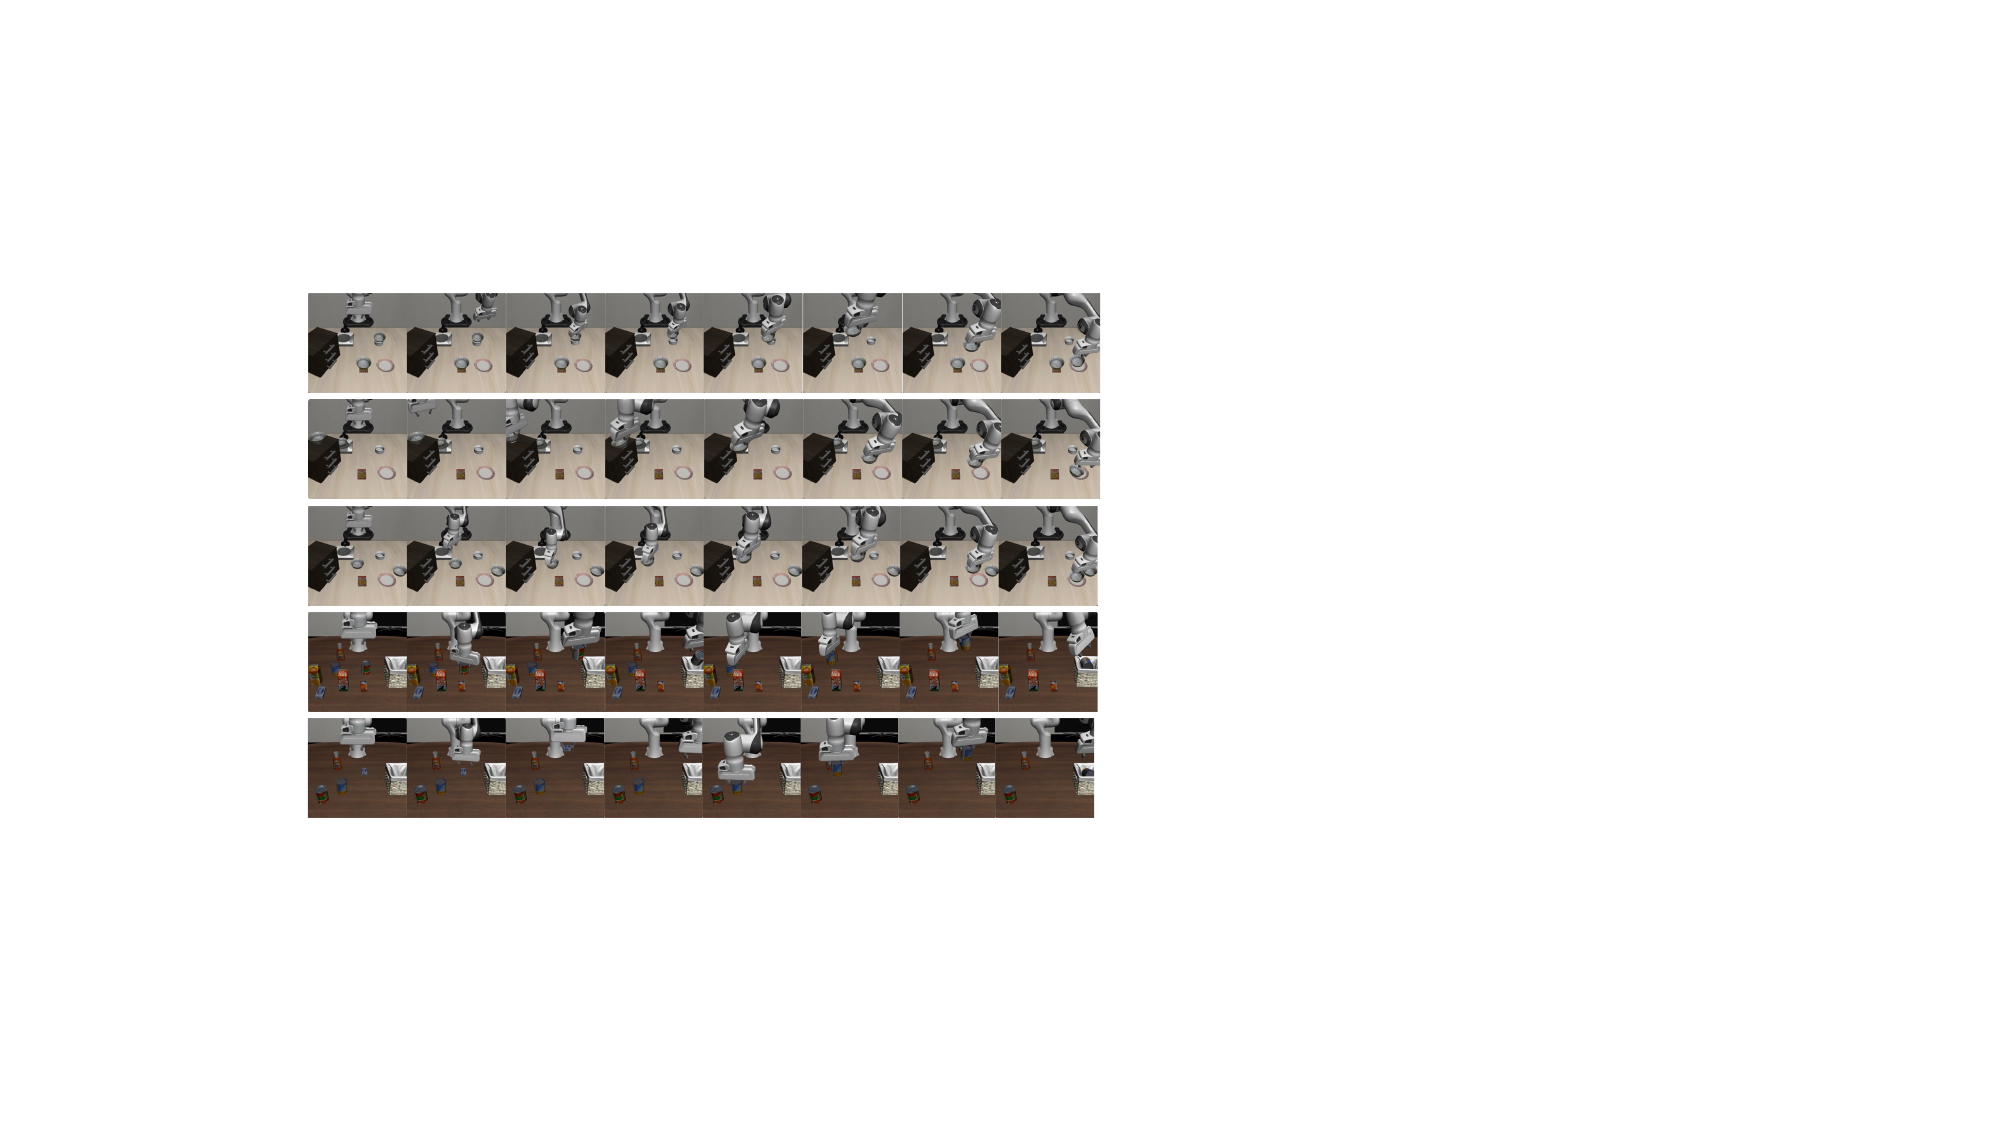}
    % \vspace{-5pt}
  \end{center}
  \caption{\textbf{More Qualitative Results.} Key frames of three task execution processes for LIBERO benchmark.}
  \label{fig:libero_qual}
  \vspace{-10pt}
\end{figure*}
