# Supplementary material for: NOD-TAMP: Generalizable Long-Horizon Planning with Neural Object Descriptors
Source: arXiv:2311.01530 source file (2024-10-05)
Supplement: Supplementary file 2 [file Appendix_.tex]

\newpage
\appendix

\subsection{Definitions}

\begin{itemize}
    \item Coordinate frame $f$
    \item World frame $w$
    \item End-effector frame $e$
    \item Movable object $o \in O$
    \item Transformation matrix $T = [R \mid t] \in \mathrm{SE}(3)$
    \item Transformation $\T{f_1}{f_2}$ from frame $f_1$ to $f_2$
    %\item Transformation $T^{f_1}_{f_2}$ from frame $f_1$ to $f_2$
    \item Frame state $S$ that contains the poses of frame $f$ relative to the world frame $w$
    \item Let $\R{S}{f_1}{f_2}$ represent the transform from frame $f_1$ to frame $f_2$ in state $S$
    %\item Frame estimates $\widehat{s}$
    \item Robot configuration $q$
    \item End-effector action $a = \T{e}{w} \in \mathrm{SE}(3)$
    \item Point cloud $P \in \mathbb{R}^{N\times3}$
    \item Segmented point cloud observation ${\cal P} = \{o:P_o \mid o {\in} P\}$
    \item NDF feature $z$
    \item Trajectory of NDF features ${\cal Z} = [z_1, ..., z_h]$
    \item Raw trajectory $\tau = [\langle S_1, a_1 \rangle, ..., \langle S_h, a_h \rangle]$ % Demonstration
    \item Frame-centric labeled trajectory $\tau = [\langle l_1, o_1, f_1, S_1, a_1 \rangle, ..., \langle l_h, o_h, f_h, S_h, a_h \rangle]$ where $l$ is the skill label, $o$ is the manipulated object $o$ and $f$ is the target frame. % Demonstration
    \item Collapse into a sequence of frame-centric trajectories ${\cal T} = [\langle l_1, o_1, f_1, \tau_1 \rangle, ..., \langle l_k, o_k, f_k, \tau_k \rangle]$
    \item Dataset of trajectories ${\cal D} = \{\tau_1, ...,  \tau_n\}$
    \item Feature trajectory $\tau = [\langle l_1, o_1, f_1, z_1 \rangle, ..., \langle l_h, o_h, f_h, z_h \rangle]$
\end{itemize}
% Frame state in world coordinates
% Maybe no actions - just use poses
% Point clouds are in world coordinates
% Can either track frames of interest and then compose through kinematics or cam track an evolving frame wrt to some cloud

\subsection{Retired}

\caelan{Any data collection assumptions about the accuracy of NDF frames?}
\caelan{Internal model of whether we're holding something}
\caelan{When holding an object, are we actually tracking a relative pose between the held object and target object (includes current grasp), or are we still just tracking the end effector?}
\caelan{Track states or actions?}

\noindent Observations:
\begin{itemize}
    \item Manipulation behavior can often be induced through (evolving) constraints on the relative transform between one or more frames, for example, grasping (static) and inserting (dynamic)
    \item We represent skills using constraints between two frames of interest
    \item Select coordinate frames that represent contact points and are more likely to generalize across a category
    \item Perfect and imperfect frame versions. Either way, frames are estimate in world coordinates, but they might not be in a canonical origin
    \item Planning should specify the frames, not just the objects
\end{itemize}

\noindent Labeled / segmented dataset:
\begin{itemize}
    \item Mimicgen: each state-action pair labeled with reference object
    \item \Ours: label interaction type and set of objects involved
    %Last, current, next contact define the labels?
\end{itemize}
\caelan{Will need to describe in the context of trajectory adaptation and planning}

\noindent Raw dataset:
\begin{itemize}
    \item RGB-D observation $o$
    \item (Training time) state $s$
    \item End-effector action $a$
    \item Trajectory $\tau = [\langle o_1, s_1, a_1 \rangle, ..., \langle o_h, s_h, a_h \rangle]$
    \item Dataset of trajectories $D = \{\tau_1, ...,  \tau_n\}$
\end{itemize}

\noindent Stuff:
\begin{itemize}
    %\item (Frame) state (estimate) $s = \{f: \T{f}{w} \mid f \in F\}$
    \item Segmented point cloud observation $o = \{f:P_f \mid f \in F\}$
    \item Frame-centric $\tau = [\langle s_1, a_1, f_1, f_1' \rangle, ..., \langle s_h, a_h, f_h, f_h' \rangle]$
    \item Tuple $\langle s, a, f, f' \rangle$ comprised of a state $s$, action $a$, target frame $f$, reference frame $f'$
    %\item For $\langle s, a, f, f' \rangle$, constraint $^{f'}T_f = (s[f'])^{-1} \cdot s[f]$ % Action is redundant
    %\item Grasped frame $f$ action $a_f = \T{e}{w}  \cdot \T{f}{e} = a \cdot \T{f}{e}$ 
    %\item Grasped frame $e$ action $a_e = ^{w}T_e  \cdot ^{e}T_e = a$ % Grasped motion generalizes
    %\item Relative transformation $s[f, f'] = ^{f'}T_f$
    \item Collapse into a sequence of frame-centric trajectories ${\cal T} = [\langle f_1, f'_1, \tau_1 \rangle, ..., \langle f_k, f'_k, \tau_k \rangle]$
\end{itemize}

\noindent Definitions:
\begin{itemize}
    %\item Frame-centric $\tau = [\langle s_1, a_1, f_1, f_1' \rangle, ..., \langle s_h, a_h, f_h, f_h' \rangle]$
    %\item State scene graph $S$ % or G
    \item Tuple $\langle S, \R{a}{e}{w}, f, f' \rangle$ comprised of a state $S$, EE action $\R{a}{e}{w}$ in world frame, target frame $f$, reference frame $f'$
    %\item End-effector action $a_w$ in the world frame $w$ % \T{e}{w}
    %\item End-effector action $a_{f'} \gets \R{S}{w}{f'} \cdot a_{w}$ in frame $f'$ 
    % \item Tool action action $a_w \gets a_w \cdot \R{S}{f}{e}$
    % \item Tool action action $a^f_w \gets a^e_w \cdot \R{S}{f}{e}$
    \item Convert into action $\R{a}{f}{f'} \gets \R{S}{w}{f'} \cdot \R{a}{e}{w} \cdot \R{S}{f}{e}$ for source frame $f$ in target frame $f'$
    \item Sequence of tuples $[\langle o, f, z\rangle_1, ..., \langle o, f, z\rangle_h]$
    % Embedding, encoding, features
    % Sequence of actions (set point vs current)?
    %\item $\proc{grasp}(o; \cdot)$: $z \gets F(\R{T}{e}{w} \mid P_o)$ % Static $P_o$
    %\item $\proc{attach}(f, f'; \cdot)$: $z \gets F(\R{T}{f}{w} \mid P_f)$
    %\item $\proc{attach}(o, f; \cdot)$: $z \gets F(\R{T}{f}{w} \mid P_o)$ % Varying $P_o$
\end{itemize}

\begin{enumerate}
    \item $\proc{transit}(\pddl{gripper}, \pddl{peg}; \tau)$: track relative pose between controlled \pddl{gripper} and uncontrolled \pddl{peg} along trajectory $\tau$.
    \item $\proc{transfer}(\pddl{peg}, \pddl{hole}; \tau)$: track relative pose between controlled \pddl{peg} (by holding) and uncontrolled \pddl{hole} along trajectory $\tau$.
\end{enumerate}
% $\proc{transit}[\pddl{gripper}, \pddl{peg}](\tau)$
% $\pddlkw{transit}[\pddl{gripper}, \pddl{peg}](\tau)$
% Interact and apply
% Grasp and attach
% Offline vs online tracking
% Change in kinematics important for planning model

\begin{equation*}
    \pi = [\proc{transit}(\pddl{gripper}, \pddl{peg}),  \proc{transfer}(\pddl{peg}, \pddl{hole})]
\end{equation*}
\begin{equation*}
    \pi = [\proc{transit}(\pddl{ee}, \pddl{peg}),  \proc{transfer}(\pddl{peg-tip}, \pddl{hole-top})]
\end{equation*}
% Any use in having transit/transfer? It might help for control affordance, but it might not be necessary for adaptation
% Evolve trajectory adaptation into operators
% If perfect tracking, no need to infer holding
% Describe more general than pick / attach?

\begin{align*}
    \pi = [&\proc{move}(), \proc{pick}(\pddl{gripper}, \pddl{peg}), \\
    &\proc{move}(), \proc{place}(\pddl{peg-tip}, \pddl{hole-top})]
\end{align*}
% Distinction between transfer / transit: moving from the pose that corresponds to the start of the next segment
% Notation for truncated segment?
% Infinitesimal trajectory reduces to pose 
% Map trajectories to sequences of relative poses
% Maybe just use transit / transfer instead of pick and place to capture temporal. Move actions as a general motion
% MoveTo vs Move (generic)

\begin{equation*}
    \pi = [\proc{grasp}[e,o_1](\tau_1), \proc{attach}[o_1,o_2](\tau_2)]
\end{equation*}
\begin{equation*}
    \pi = [\proc{grasp}_{e,o_1}(\tau_1), \proc{attach}_{o_1,o_2}(\tau_2)]
\end{equation*}
\begin{equation*}
    \pi = [\proc{grasp}^e_{o_1}(\tau_1), \proc{attach}^{o_1}_{o_2}(\tau_2)]
\end{equation*}

\begin{figure}[h]
\begin{lstlisting}
pick|$(o, g, p, q)$|
  |\kw{con}:| [|NDFGrasp$(o, g)$|, NDFPlace|$(o, p)$|, 
    |$[\proc{FK}(q)*g = p]$|]
  |\kw{pre}:| [AtPlace|$(o, p)$|, Empty|$()$|, AtConf|$(q)$|]
  |\kw{eff}:| [AtGrasp|$(o, g)$|, |$\neg$|AtPlace|$(o, p)$|, |$\neg$|Empty|$()$|]
\end{lstlisting}
\caption{TODO: Action description.}\label{fig:action}
\end{figure}
Figure~\ref{fig:action}...

\subsection{Tool Hang Example} \label{sec:example}

We will use the ``Tool Hang" task as a running example.
To complete the task, the robot must insert the \pddl{frame} object into the stand's \pddl{hole} and then hang the \pddl{tool} on the \pddl{frame}'s \pddl{handle}.
A plan that directly adapts the demonstrations might have the following form:
%\noindent NDF direct adaptation:
\begin{align*}
    \pi &= [\proc{grasp}(\pddl{frame}, \pddl{ee}; {\cal Z}_1), \proc{attach}(\pddl{frame}, \pddl{hole}; {\cal Z}_2), \\
    &\proc{grasp}(\pddl{tool}, \pddl{ee}; {\cal Z}_3), \proc{attach}(\pddl{tool}, \pddl{handle}; {\cal Z}_4)]
    % \pi &= [\proc{grasp}(\pddl{ee}, \pddl{frame}; \tau_1), \proc{attach}(\pddl{frame-tip}, \pddl{stand-hole}; \tau_2), \\
    % &\proc{grasp}(\pddl{ee}, \pddl{tool}; \tau_3), \proc{attach}(\pddl{tool-hole}, \pddl{frame-handle}; \tau_4)]
\end{align*}

Additionally, we can motions between each action in order to more robustly and efficiently move between segments. A plan that includes motion planning actions might have the following form:
%\noindent NDF + motion planning:
\begin{align*}
    \pi &= [\proc{transit}(\tau_1), \proc{grasp}(\pddl{frame}, \pddl{ee}; {\cal Z}_1), \\
    &\proc{transfer}(\pddl{frame}; \tau_2), \proc{attach}(\pddl{frame}, \pddl{hole}; {\cal Z}_2), \\
    &\proc{transit}(\tau_3), \proc{grasp}(\pddl{tool}, \pddl{ee}; {\cal Z}_3), \\
    &\proc{transfer}(\pddl{tool}; \tau_4), \proc{attach}(\pddl{tool}, \pddl{handle}; {\cal Z}_4)]
\end{align*}

\caelan{So far, assumes observability / pose estimation, so this is like a MimicGen version of the story}

\noindent Tool hang:
\begin{itemize}
    \item End-effector frame $e$
    \item Frame grasp frame $fg$
    \item Frame tip frame $ft$
    \item Stand hole frame $sh$
    \item Tool grasp frame $tg$
    \item Tool hole frame $th$
    \item Frame handle frame $fh$
\end{itemize}
\begin{align*}
    \pi = [&\proc{grasp}^e_{fg}(\tau_1), \proc{attach}^{ft}_{sh}(\tau_2), \\
    &\proc{grasp}^e_{tg}(\tau_3), \proc{attach}^{th}_{fh}(\tau_4)]
\end{align*}

\begin{algorithm}[!ht]
  \caption{Trajectory adaptation}
  \label{alg:adaptation}
  \begin{algorithmic}[1] % The number tells where the line numbering should start
    \Declare Segmented point clouds ${\cal P}$
    \Declare Frame $f$
    \Procedure{get-pose}{${\cal P}, f$}
        %\State $\widehat{S} \gets \proc{forward-kin}(\widehat{S}, q, G)$  \Comment{Update state}
        \If{$f = e$} \Comment{End-effector frame}
            \State $q \gets \proc{observe-conf}()$ \Comment{Robot conf}
            \State \Return $\proc{forward-kin}(q)$
        \EndIf
        \State \Return $\proc{ndf-estimate-pose}({\cal P}, f)$
    \EndProcedure
    \item[]
    \Declare Segmented point clouds ${\cal P}$
    \Declare NDFs ${\cal F}$
    \Declare Segmented trajectories ${\cal T}$
    \Procedure{adapt-trajectory}{${\cal P}, {\cal F}, {\cal T}$}
        \State $G \gets \{\;\}$ \Comment{Object scene graph}
        \For{$\langle o, f, {\cal Z} \rangle \in {\cal T}$}
            \For{$z \in {\cal Z}$}
                \State $\R{S}{e}{w} \gets \proc{get-pose}({\cal P}, e)$ \Comment{End-effector pose}
                \State $\R{S}{f}{w} \gets \proc{get-pose}({\cal P}, f)$ \Comment{Frame pose}
                \State $T_{z} \gets \proc{ndf-optimize}({\cal F}[o], {\cal P}[o], z)$
                \If{$o \in G$} \Comment{Relative to scene graph}
                    \State $\langle f', \R{T}{f'}{w}\rangle \gets G[o]$
                    \State $\R{S}{f'}{w} \gets \proc{get-pose}({\cal P}, f')$      
                    \State $\T{f}{w} \gets \R{S}{f'}{w} \cdot (\R{T}{f'}{w})^{-1} \cdot T_{z}$
                \Else \Comment{Relative to world frame}
                    \State $\T{f}{w} \gets T_{z}$
                \EndIf
                \State $\R{a}{e}{w} \gets \R{S}{e}{w} \cdot (\R{S}{f}{w})^{-1} \cdot \T{f}{w}$ \Comment{End-effector action}
                \State \Comment{If $f = e$, this reduces to $\R{a}{e}{w} \gets \T{f}{w}$}
                \State \Yield{} $\R{a}{e}{w}$ \Comment{Yield action to controller}
            \EndFor
            % Condition on interaction type?
            \State $G[o] \gets \langle f, \R{S}{f}{w} \rangle$ \Comment{Set $f$ as the parent of $o$}
        \EndFor
    \EndProcedure
\end{algorithmic}
\end{algorithm}

\begin{algorithm}[!ht]
  \caption{Trajectory adaptation}
  \label{alg:adaptation}
  \begin{algorithmic}[1] % The number tells where the line numbering should start
    %\Declare Initial state $S_0$
    \Declare Segmented observation $O$
    \Declare Segmented trajectories ${\cal T}$
    \Procedure{adapt-trajectory}{$S_0, {\cal T}$}
        %\State $\widehat{S}\gets S_0$ \Comment{State estimate}
        \State $G \gets \{\;\}$ \Comment{Scene graph}
        %\State $i \gets 0$
        %\For{$\langle f, f', \tau \rangle \in {\cal T}$} % Source / target
        \For{$\R{\tau}{f}{f'} \in {\cal T}$}
            %\For{$\langle s', a_w \rangle \in \tau$}
            \For{$\R{a}{f}{f'} \in \tau$}
                \State $q \gets \proc{observe-conf}()$ \Comment{Robot conf}
                %\State $\hat{S} \gets \proc{estimate-state}()$
                \State $\widehat{S} \gets \proc{forward-kin}(\widehat{S}, q, G)$  \Comment{Update state}
                \State $\R{a}{e}{w} \gets \R{\widehat{S}}{f'}{w} \cdot \R{a}{f}{f'} \cdot \R{\widehat{S}}{e}{f}$ \Comment{World frame EE action}
                \State \Yield{} $\R{a}{e}{w}$ \Comment{Yield action to controller}
                %\State $i{++}$
            \EndFor
            % Condition on interaction type?
            % Possible to unify?
            \If{$f = e$} \Comment{$\proc{grasp}(f';\cdot)$}
                \State $G[f'] \gets \langle e, \R{\widehat{S}}{f'}{e} \rangle$ \Comment{$e$ is new parent of $f'$}
                %\State $\R{\widehat{S}}{f'}{w} \gets \R{\widehat{S}}{e}{w} \cdot \R{\widehat{S}}{f'}{e}$
            \Else \Comment{$\proc{attach}(f, f';\cdot)$}
                \State $G[f] \gets \langle f', \R{\widehat{S}}{f}{f'} \rangle$ \Comment{$f'$ is new parent of $f$}
                %\State $\R{\widehat{S}}{f}{w} \gets \R{\widehat{S}}{f'}{w} \cdot \R{\widehat{S}}{f}{f'}$
            \EndIf
        \EndFor
    \EndProcedure
\end{algorithmic}
\end{algorithm}

\begin{algorithm}[!ht]
  \caption{\Ours planner}
  \label{alg:planner}
  \begin{algorithmic}[1] % The number tells where the line numbering should start
    \Declare Plan skeleton $\pi = [\langle f_1, f_1' \rangle, ..., \langle f_h, f_h' \rangle]$ % Capitalize
    \Declare Dataset ${\cal D} = \{{\cal T}_1, ..., {\cal T}_n\}$
    \Procedure{ndf-planner}{$S_0, \pi; {\cal D}$}
        \State $D_\pi = [\;]$ 
        \For{$\langle f_i, f_i' \rangle \in \pi$}
            \State $D_{f_i, f_i'} \gets \{\R{\tau}{f}{f'} \mid {\cal T} {\in} {\cal D}, \R{\tau}{f}{f'} {\in} {\cal T}.\; f {=} f_i \wedge f' {=} f_i'\}$
            \State $D_\pi \gets D_\pi + [D_{f_i, f_i'}]$
        \EndFor
        \State ${\cal T}_* \gets \None$
        \State $z_* \gets \infty$
        \caelan{Sort and filter instead of min}
        \For{${\cal T} \in \proc{combinations}(D_\pi )$} % Cartesian product, DFS
            \State $d \gets 0$
            \For{$i \in [1, ..., |{\cal T}|{-}1]$}
                \State $\langle f_i, f'_i, \tau_i \rangle \gets {\cal T}[i]$
                \State $\langle f_{i+1}, f'_{i+1}, \tau_{i+1} \rangle \gets {\cal T}[i{+}1]$
                \If{$f'_i = f_{i+1}$}
                    \State ${\cal Z}_i \gets F(\tau_i[-1] \mid P)$
                    \State ${\cal Z}_{i + 1} \gets F(\tau_{i+1}[0] \mid P)$
                    \State $d \gets d + ||{\cal Z}_{i + 1} - {\cal Z}_i||_1$
                \EndIf
            \EndFor
            \State \caelan{Goal constraints?}
            \If{$d < d_*$}
                \State ${\cal T}_* \gets {\cal T}$
                \State $d_* \gets d$
            \EndIf
        \EndFor
        %\State \Return ${\cal T}_*$
        \If{${\cal T}_* = \None$}
            \State \Return \False
        \EndIf
        \State \caelan{Motion planning}
        \State \proc{adapt-trajectory}($S_0, {\cal T}_*$)
        \State \Return \True
    \EndProcedure
\end{algorithmic}
\end{algorithm}

\begin{algorithm}[!ht]
  \caption{\Ours policy}
  \label{alg:policy}
  \begin{algorithmic}[1] % The number tells where the line numbering should start
    \Procedure{nod-tamp-policy}{${\cal T}$}
        \caelan{Unfinished}
        \For{$\langle f, f', \tau \rangle \in {\cal T}$}
            \State $o \gets \proc{observe}()$ \Comment{Observe cloud}
            \State $\widehat{s} \gets \proc{estimate}(o)$ \Comment{Estimate frame state}
            \If{$s \in S_*$}
                \State \Return \True \Comment{Success}
            \EndIf
            \State $\pi \gets \proc{plan}(s)$ \Comment{Plan}
            \For{$a \in \tau$}
                \State $\proc{execute}(a)$ \Comment{Execute action}
            \EndFor
        \EndFor
        \State \Return \True
    \EndProcedure
\end{algorithmic}
\end{algorithm}
Algorithm~\ref{alg:policy}...
